# Supplementary material for: Learning Longterm Representations for Person Re-Identification Using Radio Signals
Source: arXiv:2004.01091 source file (2020-04-02)
Supplement: Supplementary file 1 [file appendix.tex]

\section*{Appendix A: Data Collection}

\begin{figure}[h]
\vspace{-10pt}
    \centering
    \includegraphics[width=0.7\linewidth]{data-collect}

\caption{\footnotesize{The figure shows our data collection system. Orange box is our radio device to collect RF signals. Blue box is the camera to collect corresponding video for annotation and RGB baseline.}}    \label{fig:data}
\vspace{-10pt}
\end{figure}

\textbf{RF:} we use a radio device to collect RF signals (orange box in Figure 1). It contains 2 antenna arrays, one vertical and one horizontal. It uses an NVIDIA Jetson TK1 to process the data collected from the antenna arrays and upload the data to the cloud. The transmission power of the radio  is less than 1mW, which is at the same magnitude of a commercial WiFi router. The collected raw data are then processed using standard FMCW and antenna array function to generate input heatmaps and synchronized using frame rate set to 30 heatmaps per second. 

\textbf{Camera:} we use a Raspberry Pi 3 single-board computer to control the camera. The Raspberry Pi is also connected to the TK1 on the RF device to upload the video it records to the cloud. Our radio's and camera's internal clocks are synchronized using network time protocol (NTP), whose synchronization error is typically less than 10ms. 

\section*{Appendix B: Implementation Details}
\textbf{Network Architecture}: The feature extraction network from RF signal we use is similar to the one in \cite{zhao2018rf-based}. The network first uses a 12-layer spatio-temporal ResNet (3D) to aggregate the information in each RF segment. It then uses the bounding boxes provided by WiTrack \cite{adib20143d} as region proposals to crop out the region corresponding to each person. After that, another 6-layer spatial ResNet (2D) is used to extract the features from each cropped proposal. The pose-estimation sub-network for multi-task training is a 2-layer ResNet added on top of the 4-th layer of the 6-layer ResNet. Both attention blocks are multi-head attention \cite{vaswani2017attention} with 8 heads. We implement the environment discriminator with 3 fully-connected layers on top of the segment-level features.

\textbf{Training details}: during training, for each iteration we randomly sample 8 identities and 2 segments for each person to constitute a training batch. Each RF segment's horizontal heatmaps are flipped horizontally with 0.5 probability. The flipped environment is treated as a different environment than the original one when training the environment discriminator. The second attention block is trained separately on a separated training set of the training identities. 

We use Adam optimizer with learning rate 5e-4 and weight decay 5e-4. We train our model with 100 epochs in total, with a learning rate drop of 0.1 at 50 and 75 epochs (each epoch corresponds to 1000 iterations). All experiments are performed on 4 NVIDIA Titan X Pascal GPUs. During testing, RF-ReID can run in real-time with only one GPU.

\vspace{-5pt}
